# Supplementary material for: Efficient Mixture of Geographical Species for On Device Wildlife Monitoring
Source: arXiv:2504.08620 source file (2025-04-11)
Supplement: Supplementary file 1 [file appendix.tex]

\section{Appendix}

\begin{figure}[h]
  \centering
  % \fbox{\rule{0pt}{2in} \rule{0.9\linewidth}{0pt}}
   \includegraphics[width=\linewidth]{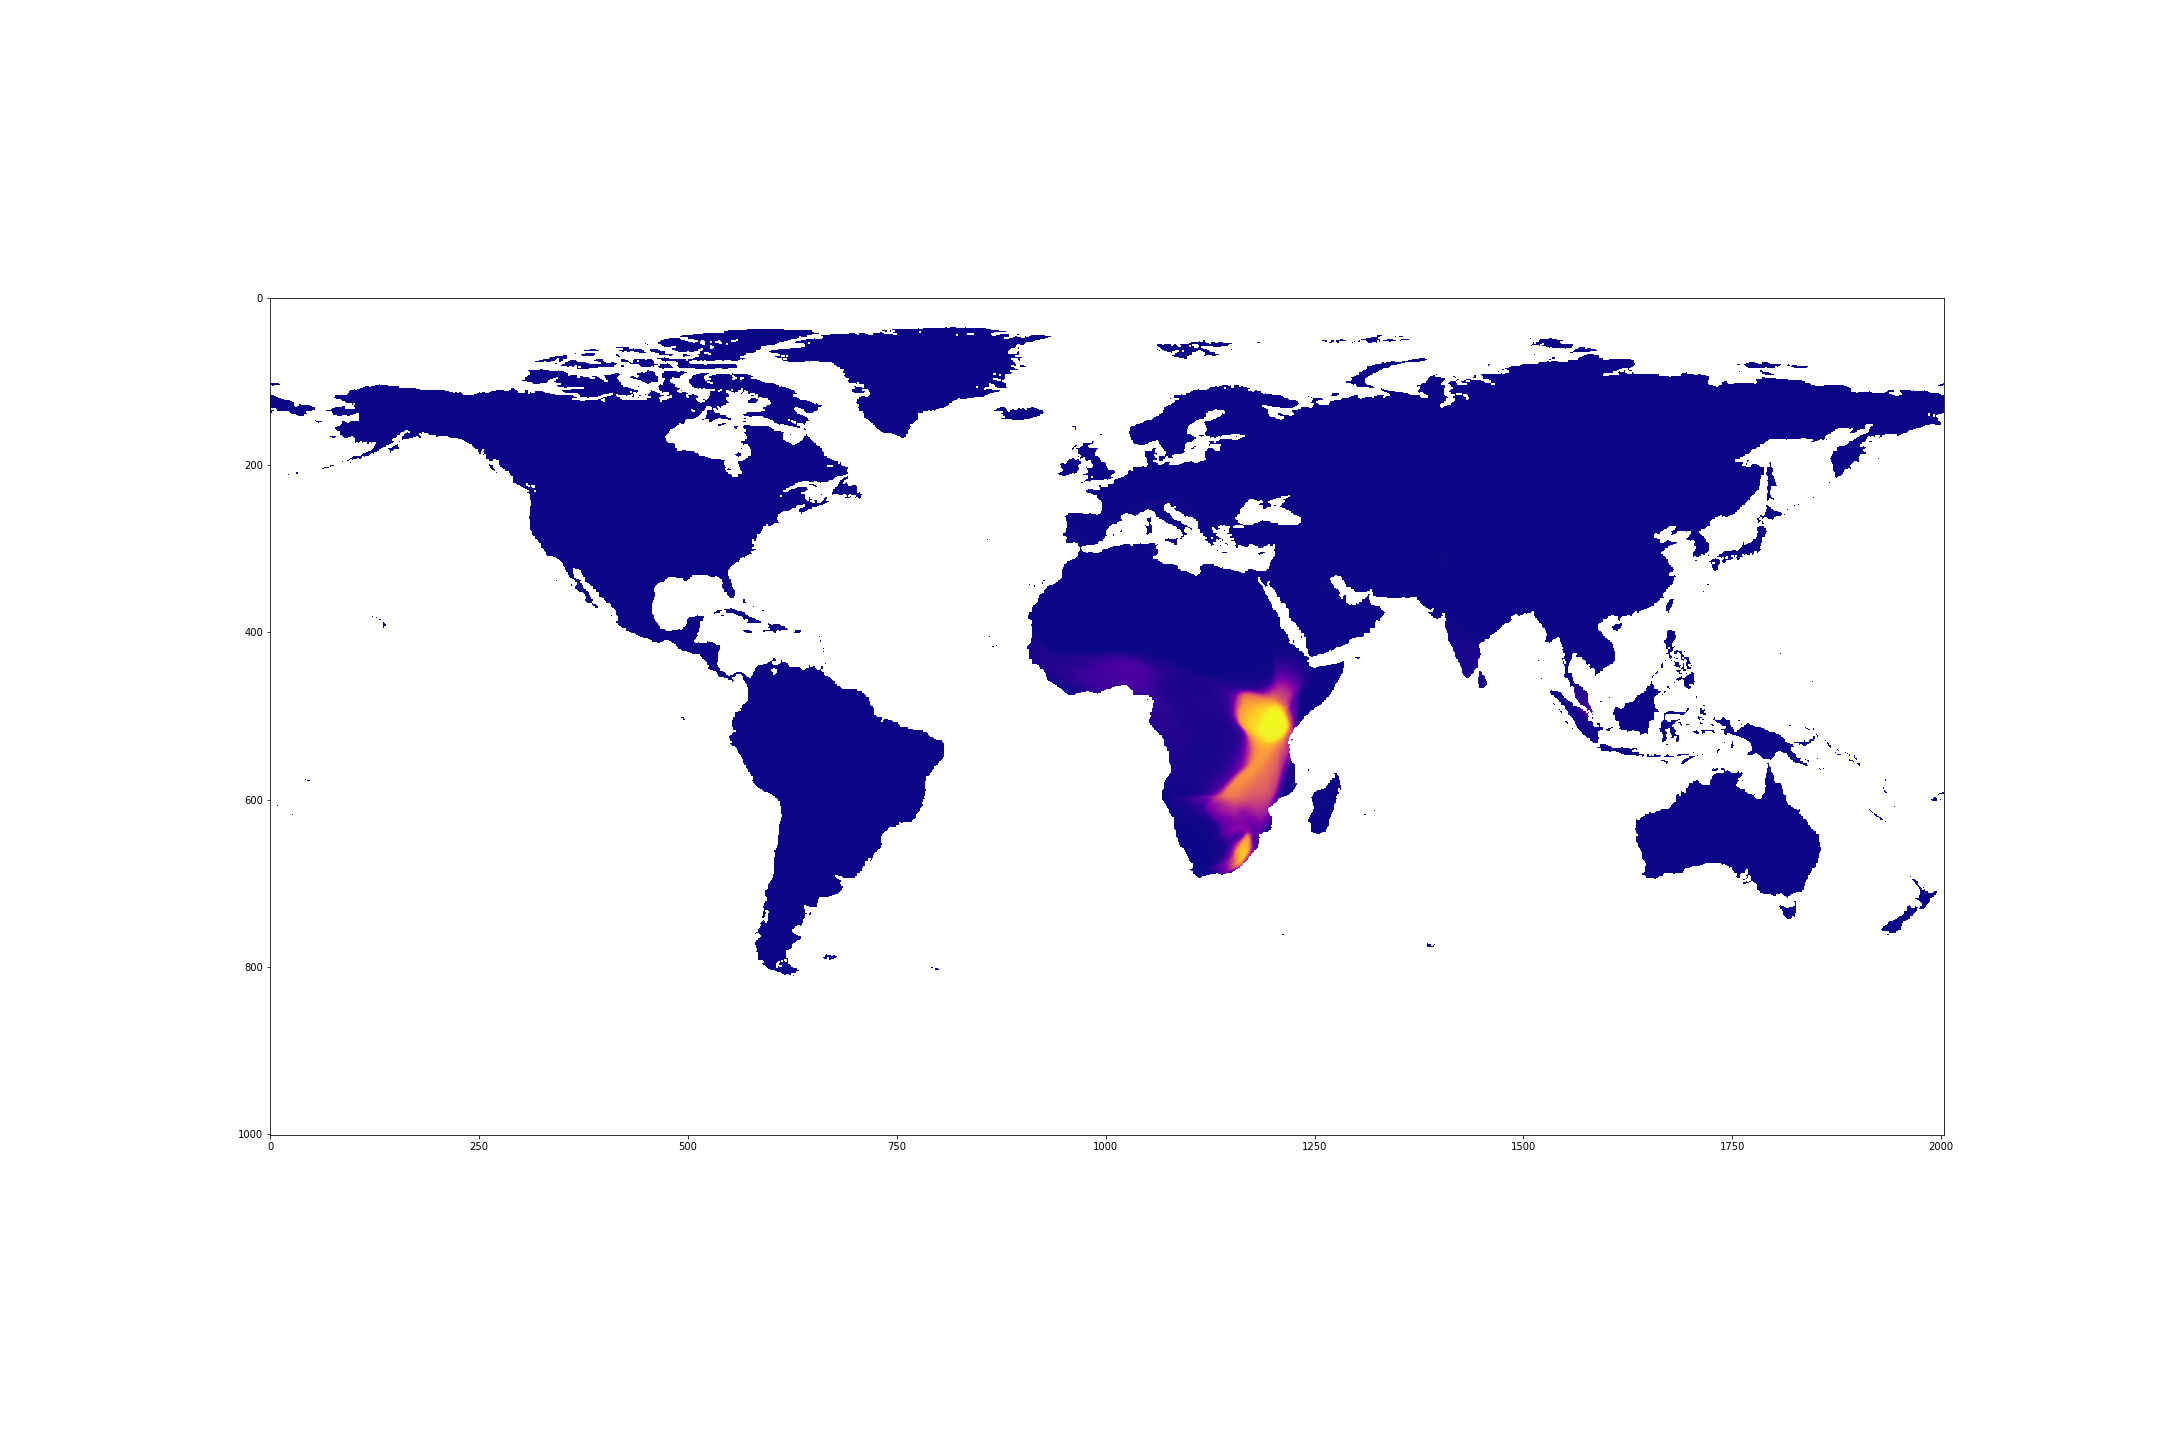}

   \caption{Sample species distribution covering about 8\% of the earth as estimated by the inaturalist species distribution prediction model [CITE]. We threshold predictions for land locations where confidence is greater than 1\% and count the fraction of land locations above this threshold.}
   \label{fig:onecol}
\end{figure}

\section{Camera Trap Global Dataset}
\label{sec:cam_trap_global}

In order to build a model that incorporates geographical information in organizing the sub-networks that will eventually determine the fraction of the full model that will remain during deployment to a given geographical location.

The inaturalist taxonomy follows the COCO format [TODO]. In order to make comparisons across datasets more meaninful, the the LILA-BC [CITE] project formats their camera trap data labels to easily map directly into the iNaturalist dataset. The table below utilizes the metadata across various camera trap datasets and the inaturalist dataset to summarize the major species represented in these datasets by count and geographical presence.

\begin{figure}[h]
  \centering
  % \fbox{\rule{0pt}{2in} \rule{0.9\linewidth}{0pt}}
   \includegraphics[width=0.8\linewidth]{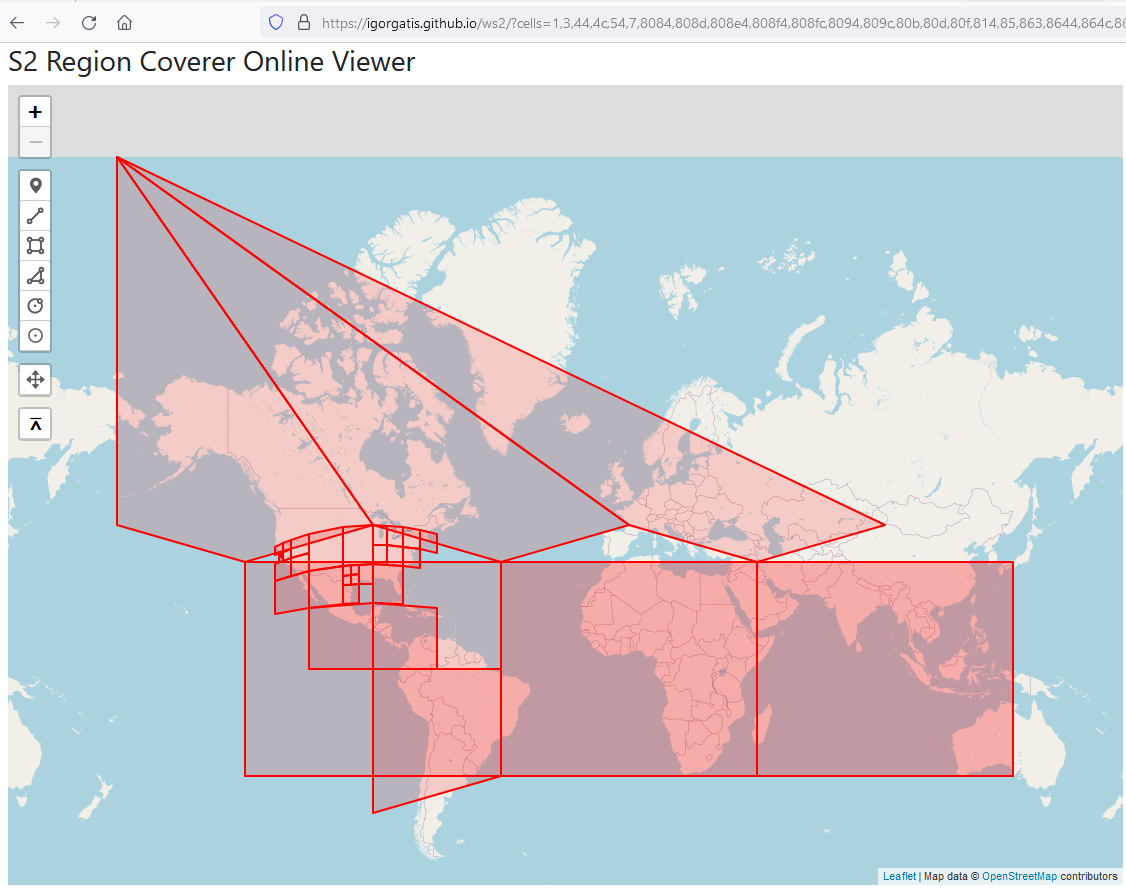}

   \caption{S2 grid division of the globe according to the federated iNaturalist 10k dataset, designed to cap the maximum number of observations for any given species within a grid in the dataset to 10 thousand observations. We augment this dataset with camera trap datasets to improve the representation of various species in the dataset as well as improve the downstream performance on camera trap deployment tasks.}
   \label{fig:onecol}
\end{figure}

\section{Expert Importance to Classification Results}
\label{sec:exp_importance}
We first begin with demonstrating how various experts in the last transformer layer (at expert level 2, 16, 64, 128) influence the classification performance of the full model on three datasets: imagenet, SSW60 on iNaturalist.

%Temporaily put here
\begin{figure}[h]
  \centering
   \includegraphics[width=0.8\linewidth]{images/inaturalist per-class accuracy bar-chart.png}

   \caption{A visualization of a per-class accuracy bar chart for three specific s2 cell locations. Our data, which was obtained from running training code and then pickling it into this notebook, is a list of tuples, where each tuple contains a list of values and a list of labels corresponding to them. Then, we loop through every tuple and then count every correct or incorrect label into an overall results array which is then plotted.}
   \label{fig:onecol}
\end{figure}

\begin{figure}
    \centering
    \includegraphics[width=1.0\linewidth]{images/hog angles/median_angles_cell_2.png}
    \caption{Median angles of HOG features for s2 cell 2/ using iNaturalist 30k dataset. Each median was calculated by taking the weighted average of the HOG vector and then taking the median of those averages.}
    \label{fig:enter-label}
\end{figure}
\begin{figure}
    \centering
n_angles_cell_4_0012.png}
    \caption{Median angles of HOG features for s2 cell 4/0012 using iNaturalist 30k dataset}
    \label{fig:enter-label}
\end{figure}

\clearpage

\section{Hyperparameter Ablation}
\label{sec:exp_importance}

Ablation studies, in the form of tables, will be placed here:

\begin{table}[!htbp]
    \centering
    \small
    \caption{Ablation for the MobileNet model, running without a focus on specific s2cells or with a pre-trained path, on 0.1 of the data for 40 Epochs.}
    \begin{tabular}{ccccc} \\ 
    \hline
     Runs & Dropout Rate &  Learning Rate & Weight Decay & Accuracy \\
     \hline
     Lemon-sweep-1 & 0 & 0.0001 & 0.00001 & \textit{\color{red}{25.308882929975223}} \\
     Fanciful-sweep-2 & 0.4 & 0.0001 & 0.0001 & \textit{\color{red}{25.26221105868775}} \\
     Classic-sweep-1 & 0 & 0.0001 & 0.00001 & \textit{\color{red}{25.449747123315568}} \\
     Noble-sweep-1 & 0.4 & 0.000001 & 0.0001 & \textit{\color{red}{25.816333457791657}} \\
     
    \hline
    \end{tabular}
    \label{tab:geo_loc_ft}
\end{table}

\begin{table}[!htbp]
    \centering
    \small
    \caption{Ablation for the MobileVit model, running on a specific collection of s2-cells without using a pre-trained path, on 0.5 of the data for 40 Epochs.}
    \begin{tabular}{ccccc} \\ 
    \hline
     Runs & Dropout Rate &  Learning Rate & Weight Decay & Accuracy \\
     \hline
     Celestial-sweep-1 & 0.3 & 0.001 & 0.00001 & \textit{\color{red}{48.883269407012655}} \\
     Balmy-sweep-2 & 0.3 & 0.0001 & 0.00001 & \textit{\color{red}{39.86456671531855}} \\
     Prime-sweep-2 & 0.5 & 0.001 & 0.00001 & \textit{\color{red}{48.50225722141136}} \\
     Rosy-sweep-2 & 0.5 & 0.001 & 0.00001 & \textit{\color{red}{48.20016292725977}} \\
     
    \hline
    \end{tabular}
    \label{tab:geo_loc_ft}
\end{table}

\begin{table}[!htbp]
    \centering
    \small
    \caption{Ablation for the MobileNet model, running on a specific subset of s2 cells without using a pre-trained path, on 1.0 of the data, for 40 Epochs.}
    \begin{tabular}{ccccc} \\ 
    \hline
     Runs & Dropout Rate &  Learning Rate & Weight Decay & Accuracy \\
     \hline
     Silvery-sweep-1 & 0.2 & 0.0001 & 0.00001 & \textit{\color{red}{39.856929500016975}} \\
     Celestial-sweep-1 & 0.2 & 0.0001 & 0.0001 & \textit{\color{red}{38.02484640711449}} \\
     True-sweep-1 & 0.2 & 0.0001 & 0.0001 & \textit{\color{red}{37.9841145921727}} \\
     Fluent-sweep-1 & 0.3 & 0.0001 & 0.0001 & \textit{\color{red}{35.915277824921084}} \\
     Logical-sweep-1 & 0.5 & 0.0001 & 0.0001 & \textit{\color{red}{34.834187570007806}} \\
     
    \hline
    \end{tabular}
    \label{tab:geo_loc_ft}
\end{table}

\begin{table}[!htbp]
    \centering
    \small
    \caption{Ablation for the MobileVit model, running without a focus on a specific subset of s2 cells or a pre-trained path, on 0.5 of the data, for 40 Epochs. Note that the first three runs ran for 39-40 epochs, while the second triplet ran for 26 epochs.}
    \begin{tabular}{cccccc} \\ 
    \hline
     Runs & Epochs & Dropout Rate &  Learning Rate & Weight Decay & Accuracy \\
     \hline
     Balmy-sweep-1 & 39 & 0.2 & 0.00001 & 0.0001 & \textit{\color{red}{15.170055327381965}} \\
     Stellar-sweep-1 & 39 &  0.2 & 0.001 & 0.0001 & \textit{\color{red}{43.056074131903195}} \\
     Silvery-sweep-1 & 39 & 0.2 & 0.001 & 0.0001 & \textit{\color{red}{19.438410101490103}} \\
     Cosmic-sweep-1 & 26 & 0.2 & 0.001 & 0.0001 & \textit{\color{red}{44.69468110383218}} \\
     Royal-sweep-1 & 26 & 0.2 & 0.0001 & 0.0001 & \textit{\color{red}{35.614880689725396}} \\
     Distinctive-sweep-1 & 26 & 0.2 & 0.00001 & 0.0001 & \textit{\color{red}{4.483893961508435}} \\
     
    \hline
    \end{tabular}
    \label{tab:geo_loc_ft}
\end{table}

\clearpage

\begin{table}[!htbp]
    \centering
    \small
    \caption{Ablation for the MobileNet model, running on a specific subset of s2 cells while using a pre-trained path, on 1.0 of the data, with the experiments set to run for 40 epochs. However, peachy failed at Epoch 27, which means we will compare values at that point}
    \begin{tabular}{ccccc} \\ 
    \hline
     Runs & Dropout Rate &  Learning Rate & Weight Decay & Accuracy \\
     \hline
     Swift-sweep-1 & 0.4 & 0.0001 & 0.0005 & \textit{\color{red}{19.54873}} \\
     Peachy-sweep-1 & 0.3 & 0.0001 & 0.0005 & \textit{\color{red}{19.88985}} \\
     Celestial-sweep-1 & 0.2 & 0.0001 & 0.0005 & \textit{\color{red}{20.05278}} \\
     
    \hline
    \end{tabular}
    \label{tab:geo_loc_ft}
\end{table}

\begin{table}[!htbp]
    \centering
    \small
    \caption{Ablation for the MobileVit model, running on a specific subset of s2 cells while using a pre-trained path, on 1.0 of the data, with the experiments set to run for 40 epochs. However, firm failed at Epoch 14, which means we will compare values at that point}
    \begin{tabular}{ccccc} \\ 
    \hline
     Runs & Dropout Rate &  Learning Rate & Weight Decay & Accuracy \\
     \hline
     Firm-sweep-1 & 0.3 & 0.001 & 0.00001 & \textit{\color{red}{54.047724109840125}} \\
     Peachy-sweep-1 & 0.3 & 0.0001 & 0.0001 & \textit{\color{red}{47.82933369539391}} \\
     Feasible-sweep-1 & 0.3 & 0.001 & 0.0001 & \textit{\color{red}{47.37704083364448}} \\
     
    \hline
    \end{tabular}
    \label{tab:geo_loc_ft}
\end{table}

\section{Sample Inaturalist Clusters}
\label{app:iwildcam_patches}

\section{Sample iWildCam Affinity }
\begin{figure*}[h]
  \centering
  % \fbox{\rule{0pt}{2in} \rule{0.9\linewidth}{0pt}}
   \includegraphics[width=0.8\linewidth]{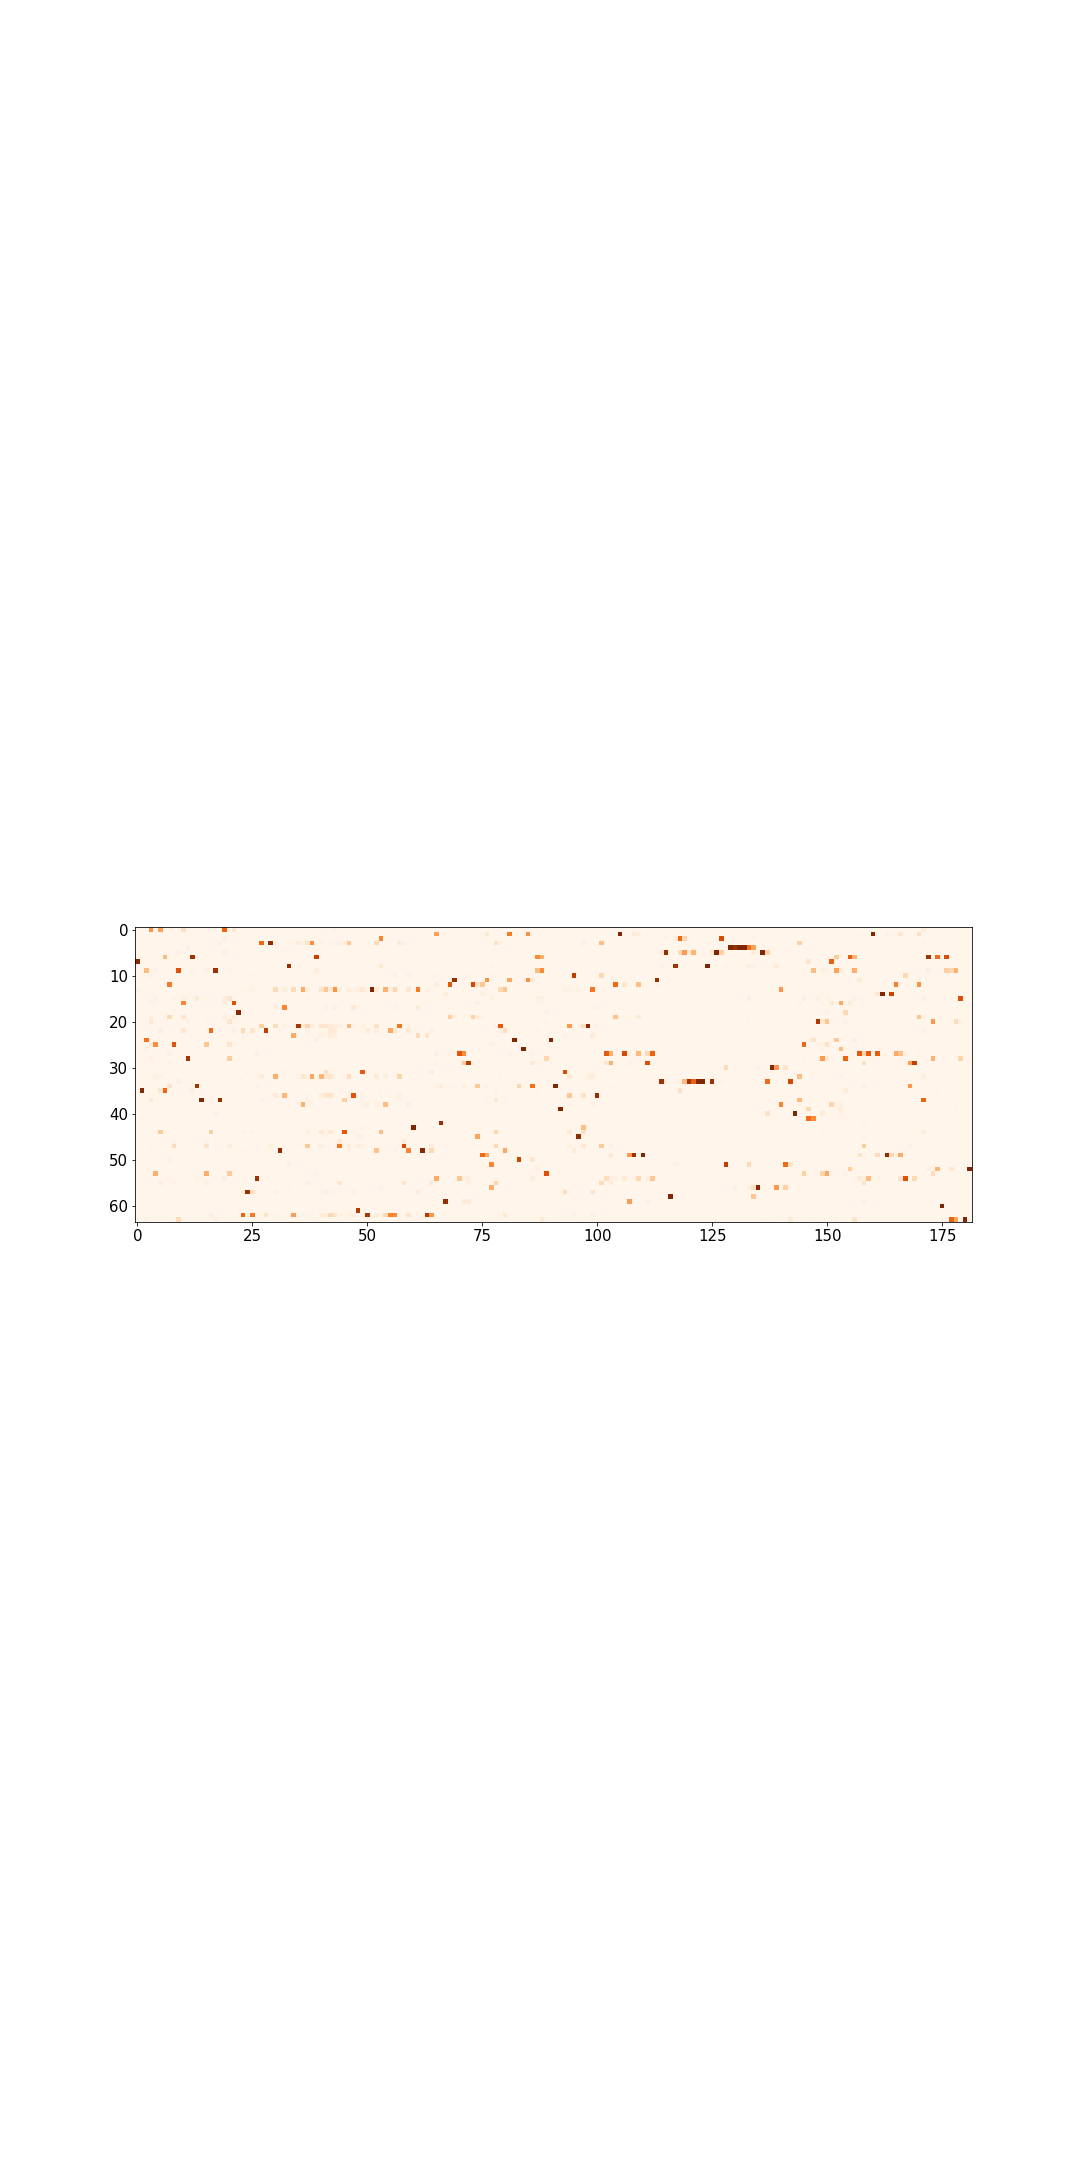}

   \caption{Affinity plot of WILDS-iWildcam train dataset at 64 experts in the last transformer block.}
   \label{fig:iwild_affinity}
\end{figure*}
\begin{figure*}[ht!]
\begin{center}
    \begin{tabular}{llll}
        \includegraphics[width=.25\linewidth]{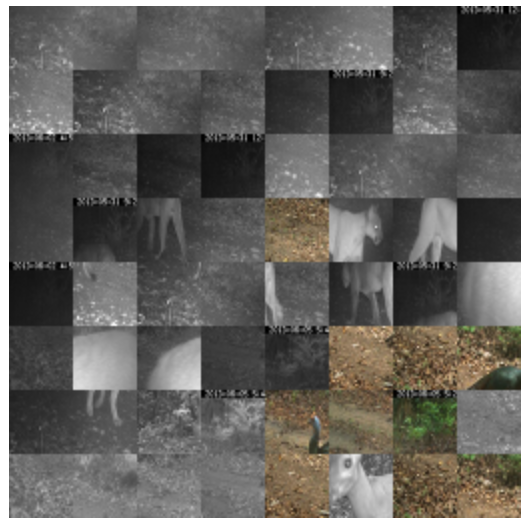} & \includegraphics[width=.25\linewidth]{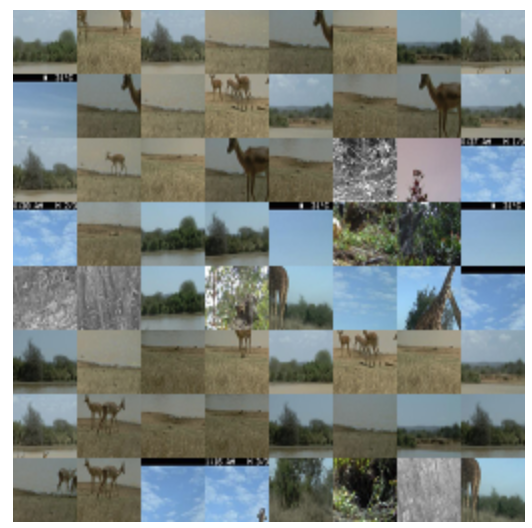} & \includegraphics[width=.25\linewidth]{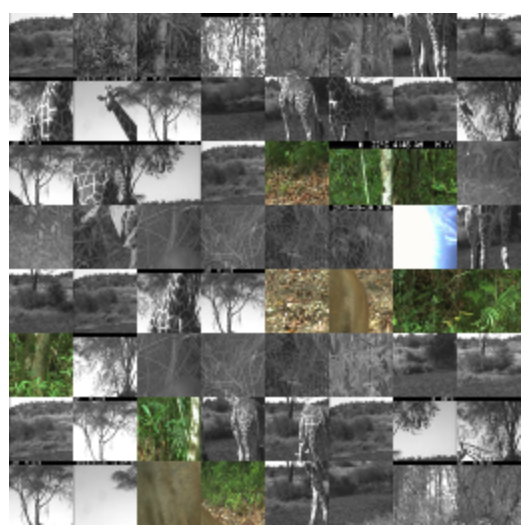}\\
        \includegraphics[width=.25\linewidth]{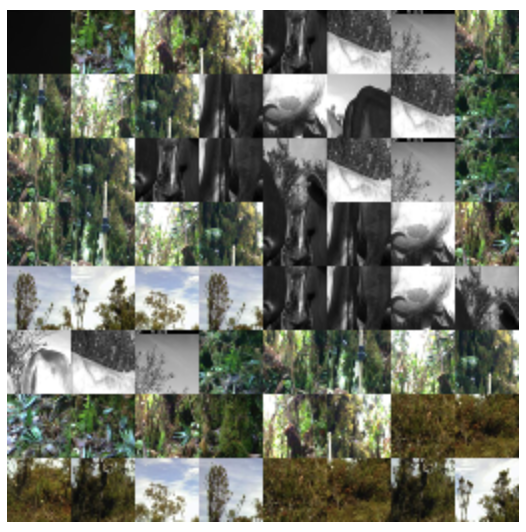} & \includegraphics[width=.25\linewidth]{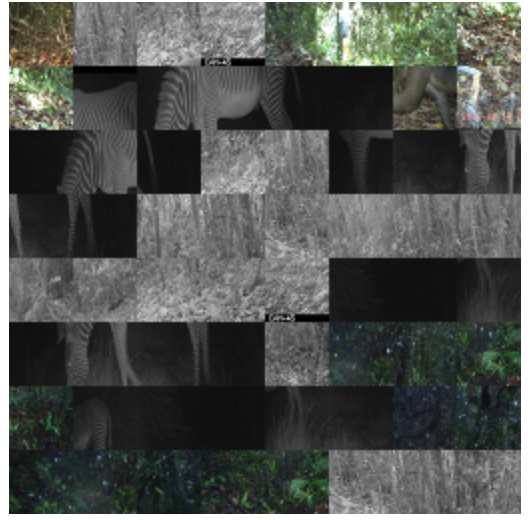} & \includegraphics[width=.25\linewidth]{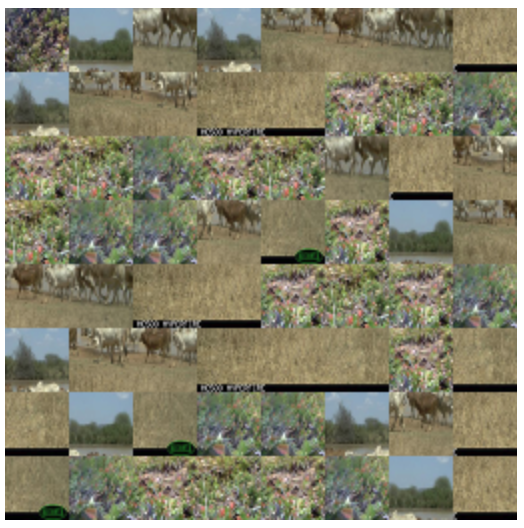}\\

        \includegraphics[width=.25\linewidth]{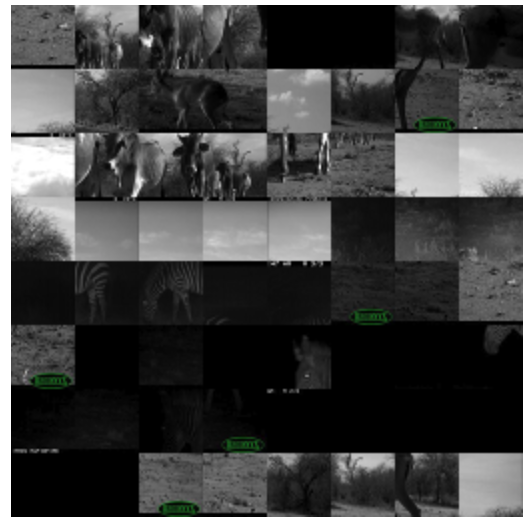} & \includegraphics[width=.25\linewidth]{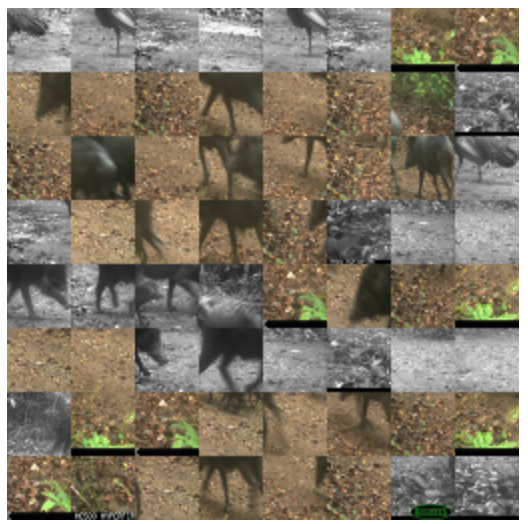} & \includegraphics[width=.25\linewidth]{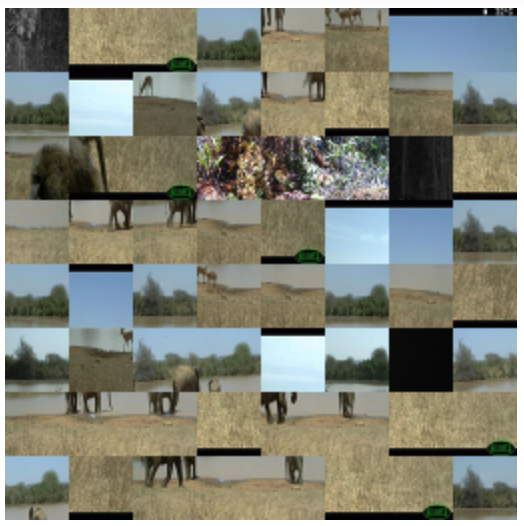}\\
        
    \end{tabular}
    
    \caption{ Sample expert groupings in the last MobileVitV2 transformer layer for WILDS-iWildcam.}
    \label{fig:iwildcam_sample_semantic_split}
\end{center}
\end{figure*}
\begin{figure*}[ht!]
\begin{center}
    \begin{tabular}{llll}
        \includegraphics[width=.25\linewidth]{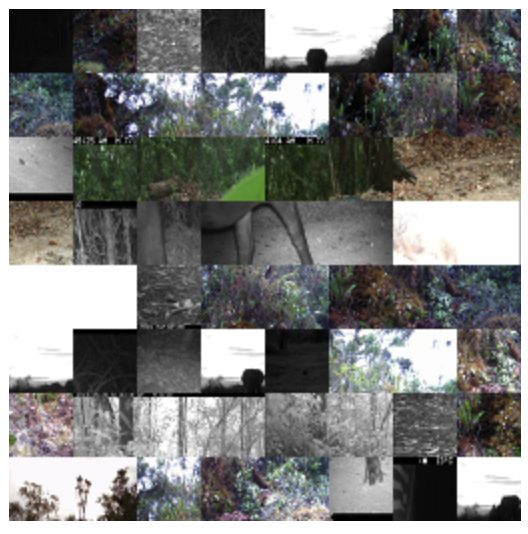} & \includegraphics[width=.25\linewidth]{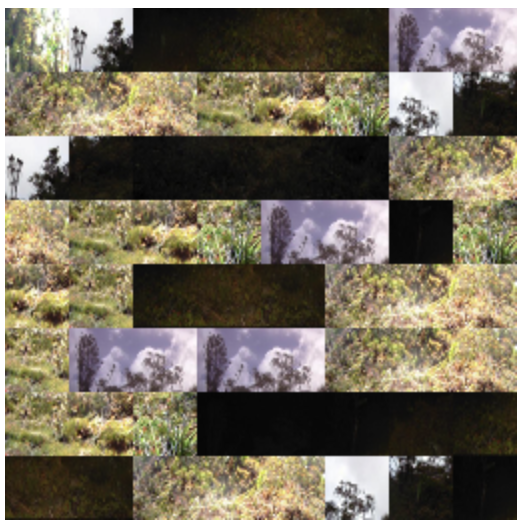} & \includegraphics[width=.25\linewidth]{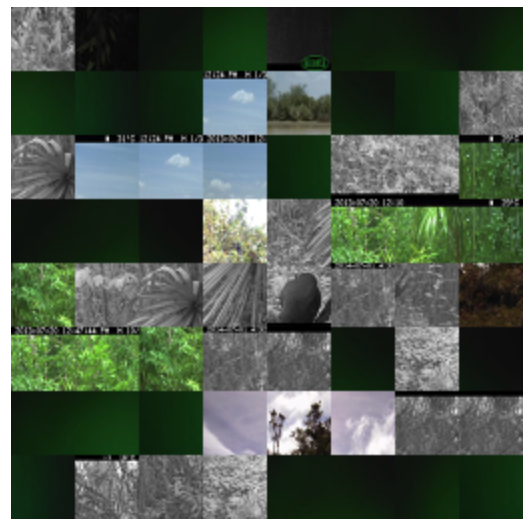}\\
        \includegraphics[width=.25\linewidth]{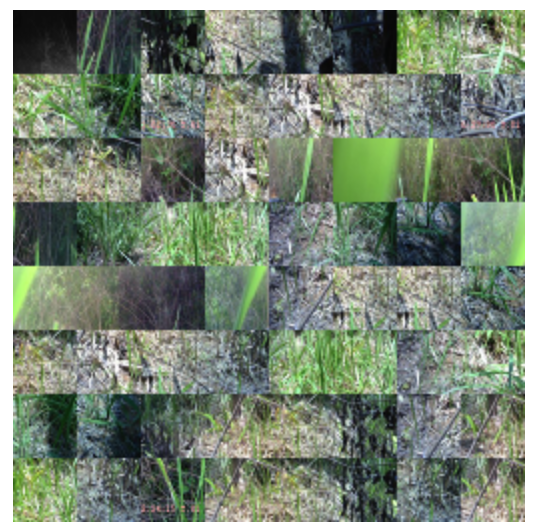} & \includegraphics[width=.25\linewidth]{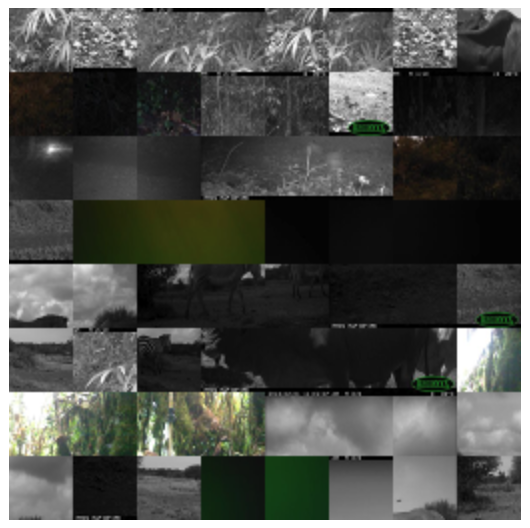} & \includegraphics[width=.25\linewidth]{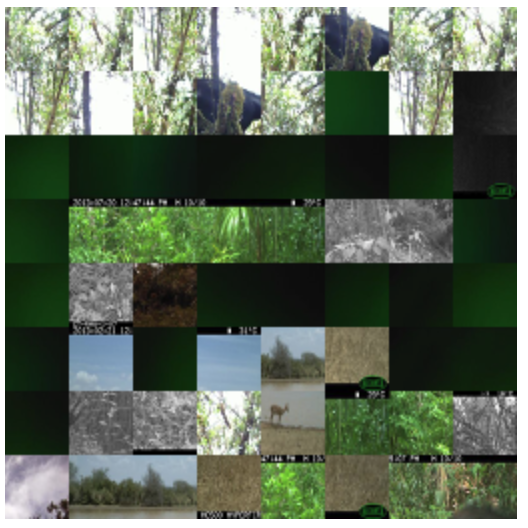}\\

        \includegraphics[width=.25\linewidth]{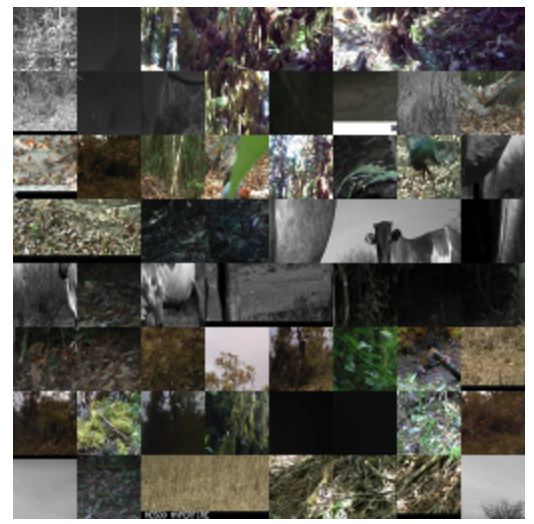} & \includegraphics[width=.25\linewidth]{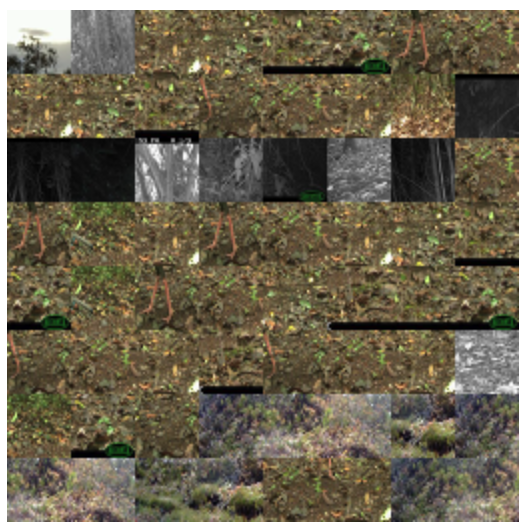} & \includegraphics[width=.25\linewidth]{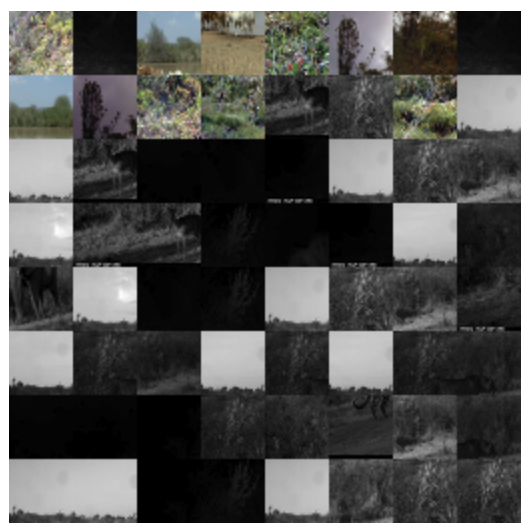}\\
        
    \end{tabular}
    
    \caption{ Sample expert groupings in the last MobileVitV2 transformer layer for WILDS-iWildcam with refining steps = $1$.}
    \label{fig:iwildcam_sample_semantic_split_ref1}
\end{center}
\end{figure*}

\section{Class level validation accuracy for WILDS-iWildcam Dataset.}
